# Supplementary material for: RoofDiffusion: Constructing Roofs from Severely Corrupted Point Data via Diffusion
Source: arXiv:2404.09290 source file (2024-10-13)
Supplement: Supplementary file 1 [file X_suppl.tex]

\clearpage
\setcounter{page}{1}
\maketitlesupplementary

\section{Rationale}
\label{sec:rationale}
Having the supplementary compiled together with the main paper means that:
\begin{itemize}
\item The supplementary can back-reference sections of the main paper, for example, we can refer to \cref{sec:intro};
\item The main paper can forward reference sub-sections within the supplementary explicitly (e.g. referring to a particular experiment); 
\item When submitted to arXiv, the supplementary will already included at the end of the paper.
\end{itemize}
To split the supplementary pages from the main paper, you can use \href{https://support.apple.com/en-ca/guide/preview/prvw11793/mac#:~:text=Delete%20a%20page%20from%20a,or%20choose%20Edit%20%3E%20Delete).}{Preview (on macOS)}, \href{https://www.adobe.com/acrobat/how-to/delete-pages-from-pdf.html#:~:text=Choose%20%E2%80%9CTools%E2%80%9D%20%3E%20%E2%80%9COrganize,or%20pages%20from%20the%20file.}{Adobe Acrobat} (on all OSs), as well as \href{https://superuser.com/questions/517986/is-it-possible-to-delete-some-pages-of-a-pdf-document}{command line tools}.

At first, we collected 16k LoD 2.2 roof mesh from \cite{virtualcitySYSTEMS_2017}. Then we analyzed the distribution of building complexity using the number of triangles and the minimum-to-maximum height variation, as shown in Figure~\ref{fig:longTail}.
The histogram reveals an imbalance in roof complexity: flat and low-complexity roofs, featuring fewer triangles, dominate the dataset. Given our focus on complex roof structures, we rebalanced the dataset by excluding 3K of the simpler roofs. This resulted in a curated dataset comprising 13K buildings.

% \subsection{Noisy Points} 
% \label{subsection:noisypoint} 
% Height maps are often susceptible to noise, originating either from the inherent sensor noise or from environmental interferences. 
% Here, we follow \cite{yu2018pu, yuan2018pcn} to emulate global noise by incorporating Gaussian noise into all the data points. 
% Additionally, we notice that height maps frequently contain outlier points, which can distort the accuracy of the data. 
% To simulate these outliers, we randomly select specific pixels and assign them random values, as suggested in \cite{zeng2022lion}.

The truth scale are also provided in the dataset for future research

\begin{itemize}
    \item data complexity distribution before/after balancing
    \item test for choosing denormalization k
    \item denormalization details
    \item tree points 
    \item line scan effect
    \item synthesize corruption details
    \item More AHN3 results 
    \item More Dales3d results
    \item More Boston results (12)
    \item More WayneCo results (12)
    \item More City3D reconstruction results
    \item failure cases
\end{itemize}
